# Supplementary material for: Privacy Budget Scheduling
Source: arXiv:2106.15335 source file (2021-06-29)
Supplement: Supplementary file 1 [file scheduling-algos-for-presentations.tex]

\setcounter{algorithm}{0}

\begin{algorithm}[!t]
    \caption{{\bf DRF} (max-min fairness over $m$ resources).}
    \begin{algorithmic}
        \State {\color{gray} \# $R = <R_1,...,R_m>$ resource capacities;}
        \State {\color{gray} \# $C = <C_1,...,C_m>$ consumed resources.}
        \Function{DominantShare}{demand vector $d_i$}
        \State return $\max_j \ \frac{d_{i,j}}{R_j}$
        \EndFunction
        \Function{onSchedulerTimer}{waiting jobs w}
        \State $\textrm{sorted\_jobs} \gets$ sortBy(\textproc{DominantShare}, w)
        \For{$i$ in  $\textrm{sorted\_jobs}$}
        \If{$C+d_i \le R$}
        \State $C=C+d_i$
        \EndIf
        \EndFor
        \EndFunction
    \end{algorithmic}
    \label{alg:drf-ppt}
\end{algorithm}

\begin{algorithm}[!t]
    \caption{{\bf DPF-N} (max-min fairness for first $N$ pipelines over $m$ private blocks).}
    \begin{algorithmic}
        \State {\color{gray} \# $R = <\epsilon^G_1,...,\epsilon^G_m>$ private blocks capacities;}
        \State {\color{gray} \# $U = <\epsilon^U_1,...,\epsilon^U_m>$ unlocked budgets.}
        \State {\color{gray} \# $C = <\epsilon^C_1,...,\epsilon^C_m>$ consumed budgets.}
        \Function{onBlockCreation}{private block $j$}
        \State $U_j\gets 0$
        \EndFunction
        \Function{onPipelineArrival}{demand vector $d_{i}$}
        \For{$\forall j: d_{i,j}>0$}
        \State $U_j \gets \min(R_j, \ U_j + \frac{R_j}{N})$
        \EndFor
        \EndFunction
        \Function{DominantShare}{demand vector $d_i$}
        \State return $\max_j \ \frac{d_{i,j}}{R_j}$
        \EndFunction
        \Function{onSchedulerTimer}{waiting pipelines w}
        \State {\color{gray} \# Similar to DRF, except ``if'' condition is: $C+d_i \le U$.}
        \EndFunction
    \end{algorithmic}
    \label{alg:dpf-ppt}
\end{algorithm}
