# Supplementary material for: Privacy Budget Scheduling
Source: arXiv:2106.15335 source file (2021-06-29)
Supplement: Supplementary file 2 [file remaining-evaluation.tex]

% See artifact.tex instead
